# Supplementary material for: Explaining Deep Neural Networks
Source: arXiv:2010.01496 source file (2021-10-13)
Supplement: Supplementary file 1 [file appendix_attention.tex]

\chapter{Architecture of \exptwoattention} 
\label{appendix-attention}

The attention model \exptwoattention{} is composed of two identical but separate modules for premise and hypothesis. The number of attended tokens is fixed to $84$, which is the maximum length of a sentence in SNLI. Here, $h_t^p$ and $h_t^h$ denote the bidirectional embeddings of the premise and hypothesis, respectively, at timestep $t$. Also, $h_{\tau}^{\text{dec}}$ denotes the decoder hidden state at timestep $\tau$, which is the context of the attention.

I use three couples of linear projections followed by $\text{tanh}$ non-linearities as follows:

I project each timestep of the encoder for premise and hypothesis:
$$ \text{proj1}_t^p = \text{tanh}(W^1_p h_t^p + b^1_p) $$ $$\text{proj1}_t^h = \text{tanh}(W^1_h h_t^h + b^1_h). $$

I separately project the context vector, that is, the hidden vector of the decoder at each timestep, before doing its dot product with the tokens of the premise and hypothesis:
$$proj_{\tau}^{c, p} = \text{tanh}(W^c_p h_{\tau}^{\text{dec}} + b^c_p) $$ 
$$ proj_{\tau}^{c, h} = \text{tanh}(W^c_h h_{\tau}^{\text{dec}} + b^c_h).$$

At each \text{dec}oding timestep $\tau$, we do the dot product between the projections of the context with all the timesteps of the premise and hypothesis, respectively:
$$ \widetilde{w_t}^{p, \tau} = <proj_{\tau}^{c, p} , \text{proj1}_t^p> $$ 
$$ \widetilde{w_t}^{h, \tau} = <proj_{\tau}^{c, h} , \text{proj1}_t^h>. $$

The final attention weights are computed from a softmax over the non-normalized weights:
$$ w_t^{p, \tau} = Softmax(\widetilde{w_t}^{p, \tau}) $$ 
$$w_t^{h, \tau} = Softmax(\widetilde{w_t}^{h, \tau}).  $$

We use another couple of projections for the embeddings of the tokens of premise and hypothesis, before we apply the weighted sum. 
$$ proj2_t^p = \text{tanh}(W^2_p h_t^p + b^2_p) $$ $$ proj2_t^h = \text{tanh}(W^2_h h_t^h + b^2_h). $$

Finally, we compute the weighted sums for premise and hypothesis:

$$ p_{\tau} = \sum_t w_t^{p, \tau} proj2_t^p$$ 
$$h_{\tau} = \sum_t w_t^{h, \tau} proj2_t^h.
 $$

At each timestept $\tau$, we concatenate $p_{\tau}$ and $h_{\tau}$ with the word embedding from the previous timestep $\tau - 1$ and give as input to our \text{dec}oder.
